# Supplementary material for: PersonaTAB: Predicting Personality Traits using Textual, Acoustic, and Behavioral Cues in Fully-Duplex Speech Dialogs
Source: arXiv:2505.14356 source file (2025-05-20)
Supplement: Supplementary file 1 [file appendix.tex]

\appendix

\section{Full Prompts for LLM}
\label{sec:appendix}

\begin{figure*}[!htb]
\begin{AIbox}{Full Prompt for Backchannel Classification}
%\begin{AIbox}{}
\small
Your task is to classify the type of backchannel. There are two types of responses: turn-taking and interjections. We focus on interjections. We have two types of encouraging interjections (back-channel): emotive and cognitive.\\
The backchannel responses are feedbacks given while someone else is talking, to show interest, attention and/or a willingness to keep listening.\\
Therefore, the interjections are not backchannels if the listener attempts to claim the speaking turn. \\

The Emotive class is one of the backchannel response, which is used to express the speaker's emotional state. The Cognitive class is another backchannel response used to reflect the speaker's thought processes or cognitive states. Your task is to classify the following interjection, delimited by triple backticks, into ``emotive", ``cognitive", ``not backchannel". \\
The texts delimited by triple backticks contain the dialog and the target text response with '(TARGET)'. \\
Triple curly blankets indicate the position of the interjection. \\

You also need to determine ``sentiment" and ``emotion" of the target interjection.
``sentiment" has 5 classes: `very positive', `positive', `neutral', `negative', and `very negative'.
``emotion" has 5 classes: `neutral', `sad', `angry', `happy', and `surprised'.

\textasciigrave\textasciigrave\textasciigrave\\
Target interjection text: yeah\\
The speaker who speaks the text inside triple curly blankets: A\\

Speaker B: yeah exactly i am like all you can eat all [StartLaugh] day long\\
Speaker A: [Laugh]\\
Speaker B: because it is open [EndLaugh] day right so you \{\{\{(TARGET) Speaker A: yeah\}\}\} can just sort of walk in i used to go you know we used to go at 11 when it first opened and then eat for like an hour you know and then talk to like two and then eat again\\
Speaker B: [Laugh]\\
Speaker A: [StartLaugh] that's a way to get your money's [EndLaugh]\\
\textasciigrave\textasciigrave\textasciigrave\\

Your response must include the classification result in JSON format at the end of the response.\\
You must perform analysis via following steps:\\
1. Summarize conversation before and after the target response.\\
2. Notice the target text.\\
3. Determine whether the target text information is backchannel or not.\\
4. [if backchannel] Determine whether the backchannel is emotive or cognitive. Note that if it's not backchannel, `interjection type' becomes `not backchannel'.\\
5. Classify ``interjection type"\\
6. Classify ``emotion" and ``sentiment"\\
This is an example of JSON:\\
\{\\
`interjection text': ``yeah",\\
`interjection type': ...,\\
`emotion': ...,\\
`sentiment': ...,\\
\}\\
\end{AIbox}
\caption{
caption
}
\label{fig:prompt_backchannel_classification}
\end{figure*}

\begin{figure*}[!htb]
\begin{AIbox}{Full Prompt for Character Prediction}
%\begin{AIbox}{}
\small
Your task is to classify the "Character" of the speaker in conversation using the Big Five Inventory (BFI) Personality Traits. BFI includes five features: openness, conscientiousness, extraversion, agreeableness, and neuroticism, detailed as follows. We also display the opposite term for each class:\\
- ``openness": intellectual, imaginative, independent-minded; opposite term is ``closedness".\\
- ``conscientiousness": orderly, responsible, dependable; opposite term is ``lack of direction".\\
- ``extraversion": talkative, assertive, energetic; opposite term is ``introversion".\\
- ``agreeableness": good-natured, cooperative, trustful; opposite term is ``antagonism".\\
- ``neuroticism": emotional instability, irritability, anxiety, self-doubt, depression; opposite term is ``emotion stability".\\

We analyzed the real conversation between two speakers and summarized their behaviors. Your task is to classify the characters using those information and sample responses. Here, I define some words used in the analysis.\\
- ``backchannel": The backchannel responses are feedbacks given while someone else is talking, to show interest, attention and/or a willingness to keep listening. \\
- ``emotive": The emotive backchannel is used to express the speaker's emotional state. \\
- ``cognitive": The cognitive backchannel is another backchannel response used to reflect the speaker's thought processes or cognitive states. \\
- ``interjection": Interjections are the responses that interject someone to stop talking and claim the speaking turn.\\

Additionally, we also show some sample responses spoken by the target speaker. We randomly extract some samples from 12-minute conversations. We excluded special tokens like commas, periods, or question marks. \\

We put all information about the target speaker within the text delimited by triple backticks.\\

\textasciigrave\textasciigrave\textasciigrave\\
Sample Responses:\\
  Sample 1: yeah you do not have to [Laugh]\\
  Sample 2: but it's still like they are cooking it so it's not really\\
 $\vdots$\\
  Sample 20: [StartLaugh] i hope you have learned [EndLaugh] a lot more since then\\
\\
Emotions:\\
  anger: 2.8\% (average: 3.7\%)\\
  disgust: 2.8\% (average: 3.7\%)\\
  fear: 2.8\% (average: 3.1\%)\\
  joy: 13.9\% (average: 11.4\%)\\
  neutral: 69.4\% (average: 48.3\%)\\
  sadness: 2.8\% (average: 10.7\%)\\
  surprise: 5.6\% (average: 19.0\%)\\
\\
Sentiment:\\
  positive: 16.7\% (average: 12.0\%)\\
  neutral: 63.9\% (average: 58.8\%)\\
  negative: 19.4\% (average: 29.2\%)\\
\\
Basic Statistics:\\
  Number of turns: Normal\\
  Talking time per turn: Short\\
  Frequency of Laughter: Very Frequent\\
  Frequency of Emotive Backchannel: Frequent\\
  Frequency of Cognitive Backchannel: Normal\\
  Frequency of interjections: Normal\\
\textasciigrave\textasciigrave\textasciigrave\\
Your response must include the classification result in JSON format at the end of the response.\\
You must perform analysis via the following steps:\\
1. Summarize features you need to consider for predicting conversation characters.\\
2. Summarize the five conversation characters (BFI)\\
3. Determine the analyzed features related to each conversation character.\\
4. Summarize the sample responses.\\
5. Summarize the emotion distribution.\\
6. Summarize the sentiment scores\\
7. Summarize the basic statistics.\\
8. Classify the five conversation features with five options ``highly aligned", ``aligned", ``neutral", ``opposed", ``highly opposed". Give ``opposed" or ``highly opposed" if the character is more aligned with the opposite terms.
\end{AIbox}
\caption{
caption
}
\label{fig:prompt_character_prediction}
\end{figure*}

\section{Subjective Evaluation}
- detail of the participants
- Website Appearance

\section{Intermediate Results}
\subsection{Dialog Generation}
- turn-taking table
- backchannel table with backchannel prediction
    - especially for the backchannels outside the predefined set
\subsection{Character Prediction}
- speaker's characteristics table including text-based conversation features

\section{Hyper-Parameters}

- Dialog Generation
    - Whisper
        - condition\_on\_previous\_text=False
        - tempareture=0.0
- Librosa silent section removal

\section{Implementation}
Implementation: LLaMa-Factory\footnote{https://github.com/hiyouga/LLaMA-Factory}

modifications:
    - model architecture
        - [ok] add input and output channels
    - dataset extraction
        - [ok] multiple channel inputs
    - loss calculation
        - [ok] multiple output channels and the loss computation is applied to only some dimensions of input
